# Supplementary material for: Fast and efficient demultiplexing of single photons from a quantum dot with resonantly enhanced electro-optic modulators
Source: arXiv:2203.08682 ancillary file (2022-03-16)
Supplement: Supplementary file 1 [file supplementary_material.pdf]

# SUPPLEMENTARY MATERIAL:

## Fast and efficient demultiplexing of single photons from a quantum dot with resonantly enhanced electro-optic modulators

Julian Münzberg,[1,a] Franz Draxl,[1] Saimon Filipe Covre da Silva,[2] Yusuf Karli,[1] Santanu Manna,[2] Armando Rastelli,[2] Gregor Weihs,[1] and Robert Keil[1]

[1] *Institut für Experimentalphysik, Universität Innsbruck, Technikerstr. 25, 6020 Innsbruck, Austria*

[2] *Institute of Semiconductor and Solid State Physics, Johannes Kepler University Linz, 4040 Linz, Austria*

(Dated: 16 March 2022)

[a] Electronic mail: julian.muenzberg@uibk.ac.at

## S1. SAMPLE STRUCTURE

The investigated sample was grown in a molecular beam epitaxy system using droplet etching epitaxy.[1] The $\lambda$-cavity consists of a $\lambda/2$ (128 nm) thick layer of $Al_{0.4}Ga_{0.6}As$ centered between two $\lambda/4$ (63 nm) thick $Al_{0.2}Ga_{0.8}As$ layers. The QD layer is placed approximately at the center in the antinode of the electric field. The central layer sits on top of a distributed Bragg reflector (DBR) consisting of 8.5 pairs of $\lambda/4$ (72 nm) thick $Al_{0.95}Ga_{0.05}As$ and $\lambda/4$ (63 nm) thick $Al_{0.2}Ga_{0.8}As$ and below two pairs of the same material combination. The sample is capped with a 4 nm thick GaAs protective layer.[2]

## S2. EOM-PBS TRANSMISSION FUNCTION

The transmission through the polarizing beam splitter (PBS) as a function of an applied voltage $V$ to the electro-optic modulator (EOM) reads (Malus' law)

$$T(V) = \sin^2\left(\frac{\pi}{2}\frac{V}{V_\pi}\right). \tag{S1}$$

We apply a sinusoidal voltage with amplitude $V_\pi/2$ to the EOM and insert a quarter-wave plate (QWP) oriented at 45° (equivalent to biasing the EOM at $V_\pi/2$) such that the voltage $V$ as a function of time $t$ is given by

$$V(t) = \frac{V_\pi}{2}\left[1 + \sin\left(2\pi f_{\mathrm{EOM}} t\right)\right]. \tag{S2}$$

By inserting Eq. (S2) into Eq. (S1), we obtain

$$T(t) = \sin^2\left(\frac{\pi}{4}\left[1 + \sin\left(2\pi f_{\mathrm{EOM}} t\right)\right]\right), \tag{S3}$$

which is plotted in Fig. S1 for $f_{\mathrm{EOM}} = 38.1\,\mathrm{MHz}$.

## S3. DAMPED RABI OSCILLATION MODEL

To retrieve the population $\eta_{\mathrm{pop}}$ at $\pi$-pulse excitation, we fit the data in Fig. 2(b) of the main manuscript according to an empirically obtained fitting function.[3,4] According to this, the probability $|c_e(\Theta)|^2$ of finding the quantum dot in the excited state $|e\rangle$ in dependence of the pulse area $\Theta \propto \sqrt{P}$ is given by

$$|c_e(\Theta)|^2 = \frac{1}{2}\left[1 - \exp\left(-\gamma\Theta\right)\cos\left(\Theta\right)\right], \tag{S4}$$

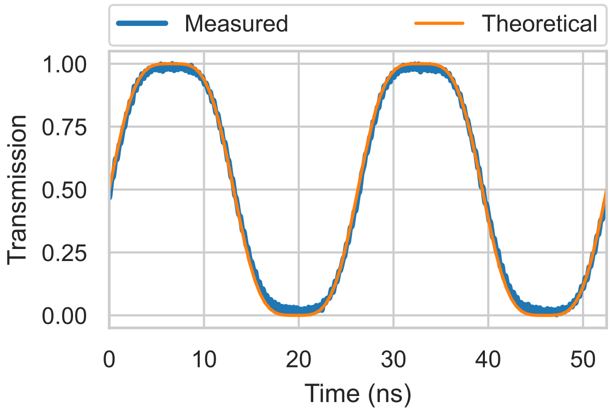


FIG. S1. Measured and theoretical transmission function of the EOM-PBS for $f_{\mathrm{EOM}} = 38.1\,\mathrm{MHz}$.

with the pulse-area-dependent damping constant $\gamma$. By introducing an amplitude re-scaling factor $A$ and substituting $\Theta = m\sqrt{P}$ with the fit parameter $m$, as well as $\gamma' = m\gamma$, we retrieve the fitting function

$$R_{\mathrm{det}}(\sqrt{P}) = \frac{A}{2}\left[1 - \exp\left(-\gamma'\sqrt{P}\right)\cos\left(m\sqrt{P}\right)\right]. \tag{S5}$$

Then, we obtain the population probability $\eta_{\mathrm{pop}}$ from the fit as the ratio of the first maximum of the fit to the amplitude $A$ of the fit:

$$\eta_{\mathrm{pop}} = \frac{\mathrm{Max}(R_{\mathrm{det}})}{A}. \tag{S6}$$

## S4. LIFETIME OF THE QUANTUM DOT

We measure the lifetime of the QD under pulsed resonant excitation of the exciton via a start-stop measurement. The signal from the internal photodiode of the pump laser serves as a start signal and the detection of a photon from the quantum dot (QD) as a stop signal. The result is shown in Fig. S2. For the measurement, we use superconducting nanowire single-photon detectors (SNSPDs) with a FWHM timing jitter of $\approx 27\,\mathrm{ps}$ and a time tagger with a FWHM timing jitter $< 24\,\mathrm{ps}$. We fit the data according to Ref. 5 and extract a fine structure splitting (FSS) of $9.7(2)\,\mu\mathrm{eV}$ and a lifetime of $167(8)\,\mathrm{ps}$.

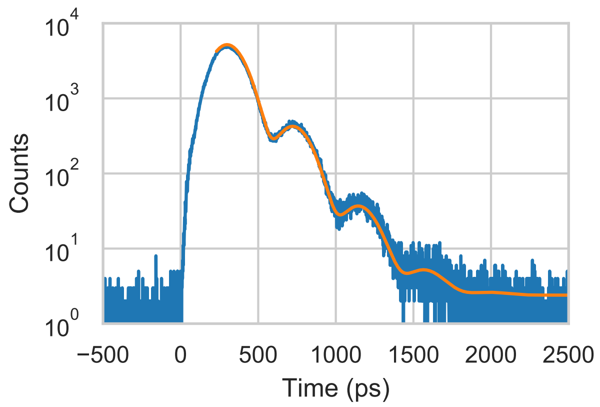


FIG. S2. Decay dynamics of the QD under pulsed resonant excitation of the exciton. The oscillation are due to the fine structure splitting of the exciton and the cross-polarized detection.[5,6]

TABLE S1. Efficiencies of the QD setup and fiber-coupled source efficiency.

| | | |
|---|---|---|
| population probability | $\eta_{\mathrm{pop}}$ | 0.909(5) |
| on-time-fraction | $\eta_{\mathrm{blinking}}$ | 0.36 |
| extraction efficiency | $\eta_{\mathrm{extr}}$ | 0.12 |
| component HWP | $\eta_{\mathrm{HWP}}$ | 0.9975 |
| component QWP | $\eta_{\mathrm{HWP}}$ | 0.9975 |
| component PBS | $\eta_{\mathrm{PBS}}$ | 0.475 |
| component GT polarizer | $\eta_{\mathrm{POL}}$ | 0.9 |
| fiber coupling efficiency | $\eta_{\mathrm{fibercoup}}$ | 0.60 |
| fiber-coupled source efficiency | $\eta_{\mathrm{QD,est}}$ | 0.010 |

## S5. QD SETUP EFFICIENCIES

We can determine the fiber-coupled source efficiency $\eta_{\mathrm{QD}}$ (compare Eq. (1) in the main manuscript) also from the estimated losses in the setup. All losses that contribute to $\eta_{\mathrm{QD}}$, as well as the estimated fiber-coupled source efficiency $\eta_{\mathrm{QD,est}}$ are summarized in Table S1. The estimated fiber-coupled source efficiency $\eta_{\mathrm{QD,est}}$ agrees reasonably well with the measured fiber-coupled source efficiency $\eta_{\mathrm{QD}}$ in Eq. (1) in the main manuscript.

The extraction efficiency from the sample is calculated from a three-dimensional finite

difference time domain simulation of the photonic structure (with the commerical software Ansys Lumerical), where we obtain $\eta_{\mathrm{extr}} \approx 0.12$ (collected into NA = 0.77) at a wavelength of 800 nm. Additionally, we estimate the fiber coupling efficiency by recording an image of the QD emission with a nitrogen-cooled camera (exposure time 120 s). For this, we excite a QD via two-photon excitation and remove the pump laser by cross-polarized excitation/collection and additional notch filters. The image data is obtained in a different optical setup but with a similar sample (same photonic structure but slightly lower emission wavelength of around 785 nm) such that the mode shape of the QD emission is expected to be comparable. In order to calculate the fiber coupling efficiency in the setup used throughout this work, we need to re-scale the image. We obtain the correct rescaling factor by performing a knife-edge measurement just before the fiber coupler in our setup, where we measure a beam diameter of 1.6 mm, such that the image can then be re-scaled to match with this beam diameter. We import the re-scaled QD image to the simulation program (VirtualLab Fusion Trial) and focus the field with an aspheric lens (Edmund Optics NT47-725, L-BAL35, f=11.25 mm, comparable focal length as the fiber coupler). We obtain a maximum coupling efficiency of 0.60 by calculating the complex overlap integral between the focused field and the fiber mode (NA= 0.12, MFD = 5.3(10) µm at 850 nm).

We expect that the simulated extraction efficiency and the calculated fiber coupling efficiency have the largest uncertainty since the fabrication parameters do not perfectly match the simulated parameters. The exciton emission frequency could be slightly displaced with respect to the cavity resonance frequency which would decrease $\eta_{\mathrm{extr}}$ and $\eta_{\mathrm{fibercoup}}$.

## S6. QUANTUM DOT BLINKING

We investigate blinking of the QD by performing a Hanbury Brown and Twiss (HBT) measurement on a millisecond timescale. The results are shown in Fig. S3(a) for resonant excitation (as used in the experiment) and in Fig. S3(b) for resonant excitation where we additionally illuminate the sample with weak above bandgap laser light at 532 nm. In the measurement, the bin width is set to 100 µs and 10 µs for Fig. S3(a) and Fig. S3(b), respectively. On a millisecond timescale, we observe bunching with $g^{(2)}(\tau) > 1$, which we attribute to blinking of the QD. We retrieve the blinking timescale from an exponential fit to the data, which is $\approx 7$ ms and $\approx 110$ µs for Fig. S3(a) and Fig. S3(b), respectively. We

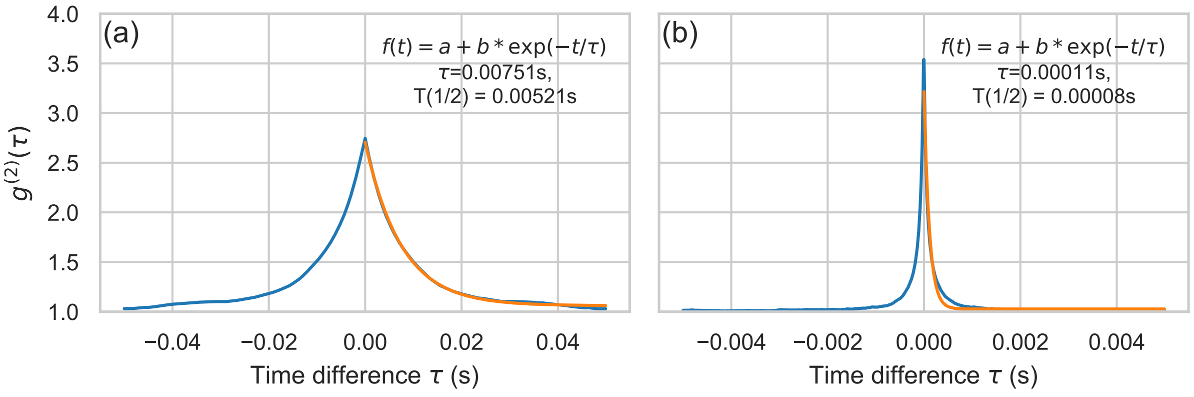


FIG. S3. Second-order intensity correlation histogram on a millisecond timescale. (a) Direct resonant excitation of the QD. (b) Direct resonant excitation of the QD with additional weak illumination at 532 nm.

calculate the on-time-fraction $\eta_{\text{blinking}}$ of the QD from $g^{(2)}(0)$[7,8]

$$\eta_{\text{blinking}} = \frac{t_{\text{on}}}{t_{\text{off}} + t_{\text{on}}} = \frac{1}{g^{(2)}(0)}, \tag{S7}$$

which is $\eta_{\text{blinking}} = \frac{1}{2.75} = 0.36$ and $\eta_{\text{blinking,AB}} = \frac{1}{3.5} = 0.28$ for resonant excitation without and with additional above bandgap laser illumination, respectively. With this specific sample and QD, additional above bandgap laser illumination therefore decreases the brightness of our single-photon source. Another reference reports the opposite effect for a GaAs QD excited via two-photon excitation (TPE), where additional white light illumination increases the on-time-fraction of the QD.[9] In both cases, above bandgap illumination accelerates the blinking dynamics. Since the most likely origin of blinking is the random capture of charges by the QD, it is evident that the above bandgap illumination increases the capture rate, which may result in both neutralization or charging of the QD and thus switching between on and off states.

## S7. TIMETRACE OF COUNT RATES

In the experiment, we measure the single-channel count rates, as well as twofold, threefold, and fourfold coincidence rates in measurement intervals (integration time) of 1 s over the course of ≈ 15 h. The data presented in Table I of the main manuscript is the average over the whole measurement time. Figure S4(a) and S4(b) show the single-channel count rates

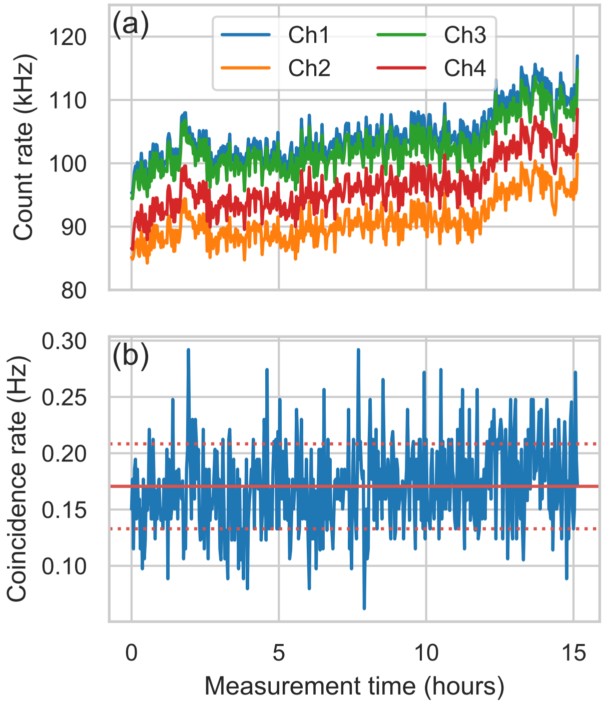


FIG. S4. (a) Measured count rates at the four output channels of the routing setup over the measurement time of the experiment. (b) Measured fourfold coincidence rate. One data point corresponds to an integration time of 120 s. The mean fourfold coincidence rate (red solid line) as well as the Poissonian counting uncertainty (red dotted lines) is indicated.

and the fourfold coincidence rate, respectively. The data is re-sampled to an integration time of 120 s per data point. After $\approx 12$ h a slight increase in the single-channel count rates is observed, which we attribute to a degradation in the laser suppression. The fourfold coincidence rate is almost unaffected.

## S8. INTERFEROMETRIC PATH LENGTH ADJUSTMENT

Optical path length differences in the four output channels of the routing setup lead to imperfect temporal overlap of the photons, which degrades the observed two-photon interference (TPI) visibility. Three of the four output couplers (channel 1, 3, and 4) are mounted on linear translation stages, such that optical path length differences in the routing setup and the optical fibers from the setup to the beamsplitter (or any other structure that implements a unitary transformation for a multiphoton interference experiment) can be

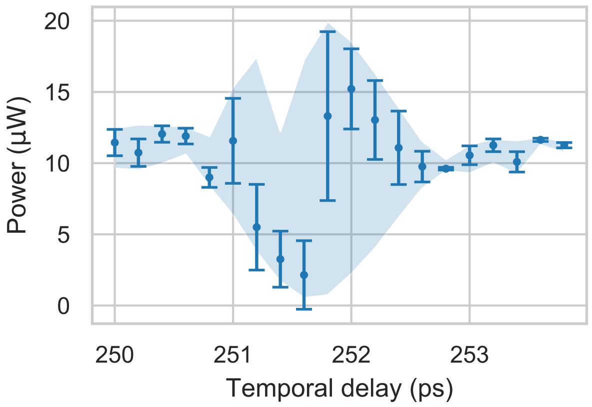


FIG. S5. Optical path length adjustment of Ch. 3 with respect to Ch. 2. We scan the temporal delay of Ch. 3 and measure the power at one output of the attached beamsplitter. For each temporal delay, we record 1000 data points with an integration time of $\approx 10\,\mathrm{ms}$. The graph shows the mean power (circle), one standard deviation (error bar), as well as the minimum and maximum value (edges of the light blue area). From the measurement, we find an optimal temporal delay of $251.65\,\mathrm{ps}$.

compensated for.

In order to adjust the optical path length of one channel with respect to another channel, we perform the following procedure (here e.g. described for Ch. 2 and 3): We attach the pulsed laser (which is otherwise used to excite the QD) directly to the input of the routing setup. For this measurement, we slightly decrease the pulse duration to $\approx$ 1-3 ps for a better temporal resolution. We connect the two output channels of the routing setup to a fiber beamsplitter (the same one as in the TPI measurement). The EOMs are turned off and the QWP before EOM A and B is replaced by a half-wave plate (HWP). The waveplate angles are adjusted so that roughly the same optical power arrives at the two output Ch. 2 and 3. In this configuration, the setup spans a Mach-Zehnder interferometer. Hence, interference fringes should be visible as the phase of one interferometer arm is scanned and, simultaneously, the two pulses temporally overlap.

We scan the linear stage of Ch. 3 (correspondingly the temporal delay) and record the power for each delay. The results are shown in Fig. S5. The phases of the two interferometer arms are not stable due to temperature changes and air turbulence such that the recorded signal fluctuates substantially due to interference of the two paths, as long as the two pulses

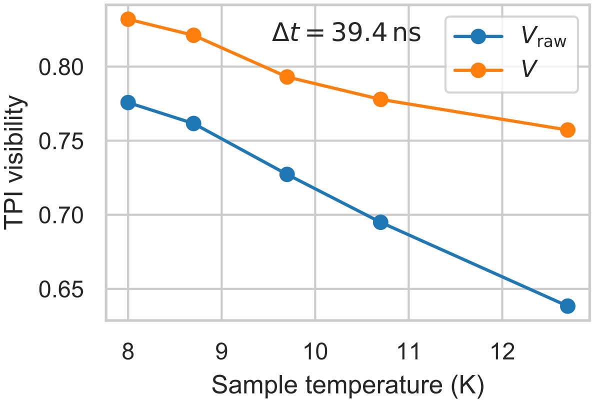


FIG. S6. TPI visibility for varying sample temperatures at a temporal delay of 39.4 ns (corresponding to output Ch. 1 and 4). $V_{\mathrm{raw}}$ is the measured visibility and $V$ is the visibility corrected for an imperfect splitting ratio and a finite $g^{(2)}(0)$ according to Eq. (4) in the main manuscript. $g^{(2)}(0)$ increases with temperature due to misalignment of the cross-polarized laser suppression.

temporally overlap. The fluctuation vanishes for no overlap. The fluctuation is largest for 251.65 ps, which corresponds to the best temporal overlap of photons from the two channels. The procedure is repeated twice in order to adjust the optical path length of the two remaining channels 1 and 4 with respect to Ch. 2.

## S9. TEMPERATURE DEPENDENCE OF TPI VISIBILITY

We measure the temperature dependence of the TPI visibility for a temporal delay of 39.4 ns. The results are shown in Fig. S6. The indistinguishability of the photons drops with increasing temperature due to phonon-induced pure dephasing. The observed raw and corrected TPI visibility at a temperature of 8 K is slightly different compared to the value reported in Sec. IV of the main manuscript. We expect that this is due to uncertainties in the measurement, since this measurement was performed during another cool down of the sample with marginally different alignment conditions and cross-polarized laser suppression (in this measurement $g^{(2)}(0)$ increased from 0.030 to 0.067 for temperatures from 8 to 12.7 K possibly due to misalignment of the cross-polarized laser suppression as the temperature changes).

## REFERENCES


[1]S. F. Covre da Silva, G. Undeutsch, B. Lehner, S. Manna, T. M. Krieger, M. Reindl, C. Schimpf, R. Trotta, and A. Rastelli, Appl. Phys. Lett. **119**, 120502 (2021).

[2]M. Reindl, J. H. Weber, D. Huber, C. Schimpf, S. F. C. D. Silva, S. L. Portalupi, R. Trotta, P. Michler, and A. Rastelli, Phys. Rev. B **100**, 155420 (2019).

[3]A. Zrenner, E. Beham, S. Stufler, F. Findeis, M. Bichler, and G. Abstreiter, Nature **418**, 612 (2002).

[4]P. L. Ardelt, L. Hanschke, K. A. Fischer, K. Müller, A. Kleinkauf, M. Koller, A. Bechtold, T. Simmet, J. Wierzbowski, H. Riedl, G. Abstreiter, and J. J. Finley, Phys. Rev. B **90**, 241404(R) (2014).

[5]E. Schöll, L. Hanschke, L. Schweickert, K. D. Zeuner, M. Reindl, S. F. C. da Silva, T. Lettner, R. Trotta, J. J. Finley, K. Müller, A. Rastelli, V. Zwiller, and K. D. Jöns, Nano Lett. **19**, 2404 (2019).

[6]H. Ollivier, I. Maillette De Buy Wenniger, S. Thomas, S. C. Wein, A. Harouri, G. Coppola, P. Hilaire, C. Millet, A. Lemaître, I. Sagnes, O. Krebs, L. Lanco, J. C. Loredo, C. Antón, N. Somaschi, and P. Senellart, ACS Photonics **7**, 1050 (2020).

[7]J.-P. Jahn, M. Munsch, L. Béguin, A. V. Kuhlmann, M. Renggli, Y. Huo, F. Ding, R. Trotta, M. Reindl, O. G. Schmidt, A. Rastelli, P. Treutlein, and R. J. Warburton, Phys. Rev. B **92**, 245439 (2015).

[8]C. Schimpf, M. Reindl, D. Huber, B. Lehner, S. F. Covre Da Silva, S. Manna, M. Vyvlecka, P. Walther, and A. Rastelli, Sci. Adv. **7**, eabe8905 (2021).

[9]C. Schimpf, M. Reindl, P. Klenovský, T. Fromherz, S. F. Covre Da Silva, J. Hofer, C. Schneider, S. Höfling, R. Trotta, and A. Rastelli, Opt. Express **27**, 35290 (2019).
